# Supplementary material for: Integration of imprint-free and low coercivity ferroelectric BaTiO3 thin films on silicon
Source: arXiv:2510.13435 source file (2025-10-15)
Supplement: Supplementary file 1 [file Supplementary_Materials_BTO.pdf]

# Supplementary Information: Integration of imprint-free and low coercivity ferroelectric $BaTiO_3$ thin films on silicon

Jingtian Zhao,[1,2] Beatriz Noheda,[1,2] and Martin F. Sarott[1,2]

[1]*Zernike Institute for Advanced Materials, University of Groningen, 9747AG Groningen, The Netherlands.*

[2]*Groningen Cognitive Systems and Materials Center (CogniGron), University of Groningen, 9747AG Groningen, The Netherlands.*

(Dated: October 13, 2025)

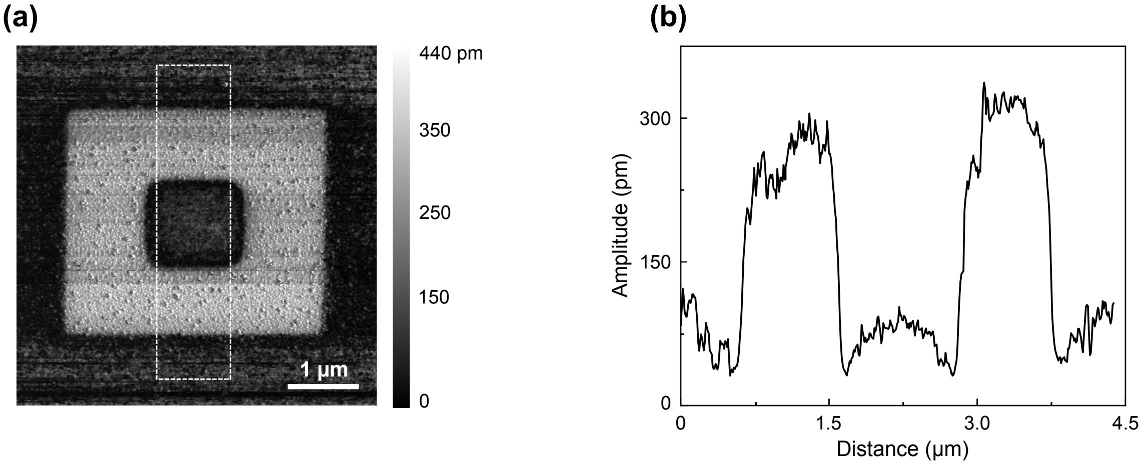


Figure S1. **Vertical PFM amplitude and averaged line profile across the poled area on BTO/SRO/SSTO/STO.** The vertically averaged line profile in (b) across the rectangular dashed outline in (a) shows a clear suppression of the vertical PFM amplitude at the location of the 180° domain wall. The enhanced PFM amplitude of the downward-poled outer box likely originates either from electrostatic charging or a slight misalignment of the laser spot on the back of the PFM cantilever.

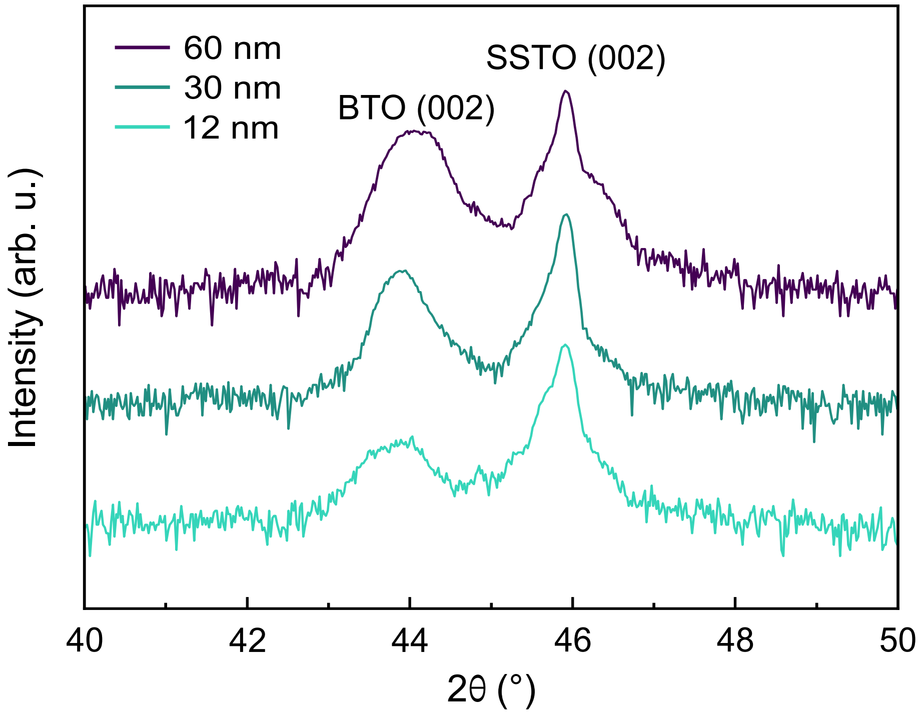


Figure S2. **Symmetric XRD $\theta$–$2\theta$ scans of the BTO/SRO/SSTO heterostructure grown on STO-buffered Si** (001) **with different thickness.** For all films, independent of thickness, the BTO tetragonality remains unchanged. We do not observe any deviations from the pure out-of-plane orientation.

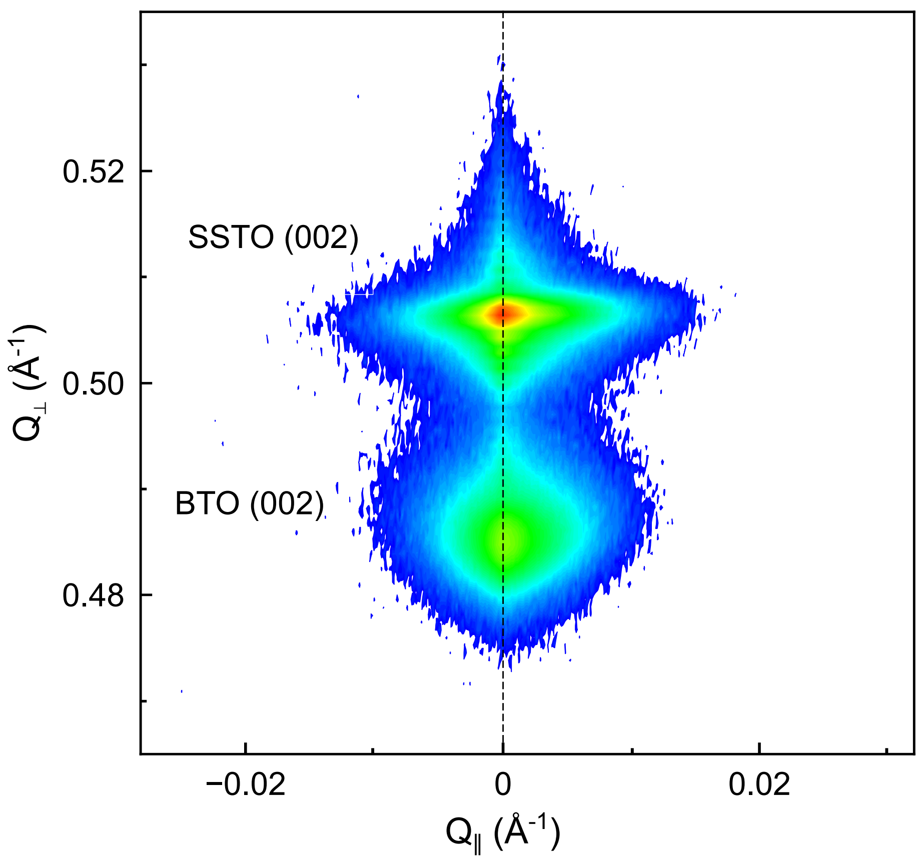


Figure S3. **XRD reciprocal space map around the symmetric BTO (002) reflection.** The absence of peak splitting along $Q_\perp$ and butterfly-shaped peak elongations around the BTO reflection, confirm the absence of a multi-$a/c$-domain configuration and point to a pure c-axis-oriented growth of our BTO on silicon.

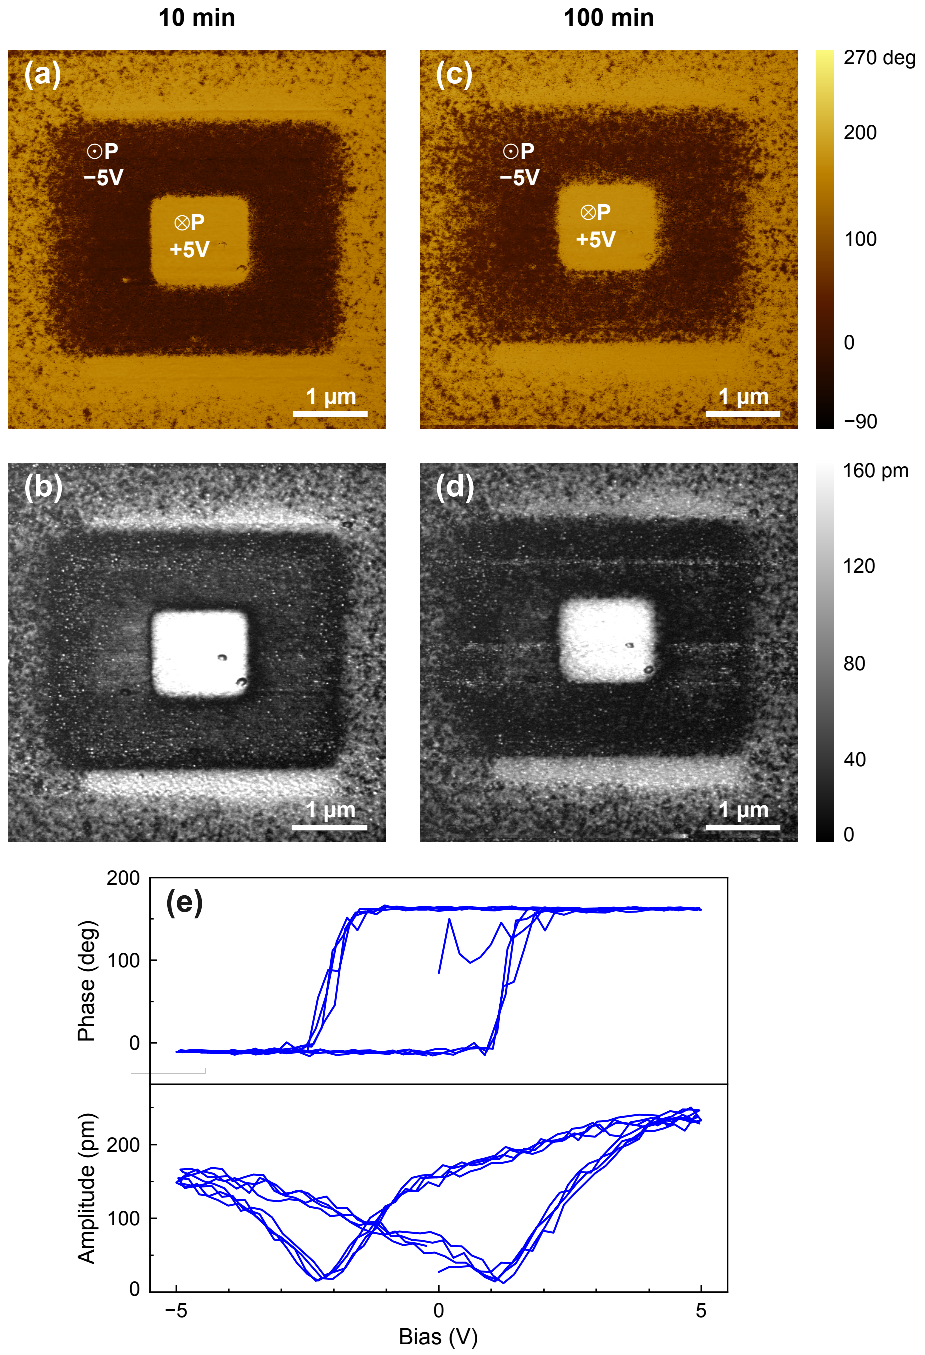


Figure S4. **PFM retention on BTO/SRO/SSTO/STO-Si.** Vertical PFM phase and amplitude (a,b) ~10 min after box-in-box poling and (c,d) ~100 min after poling. While a weakening of the amplitude and phase contrast is evident, the poled areas are retained under continuous PFM scanning for at least 100 min. Note that the areas above and below the outer poled exhibit an enhanced amplitude and uniform phase due to a previously applied positive DC voltage in this area. In the pristine state, we observe a multi-domain configuration with a predominate downward-oriented polarization. (e) PFM switching spectroscopy loops on a pristine film area.

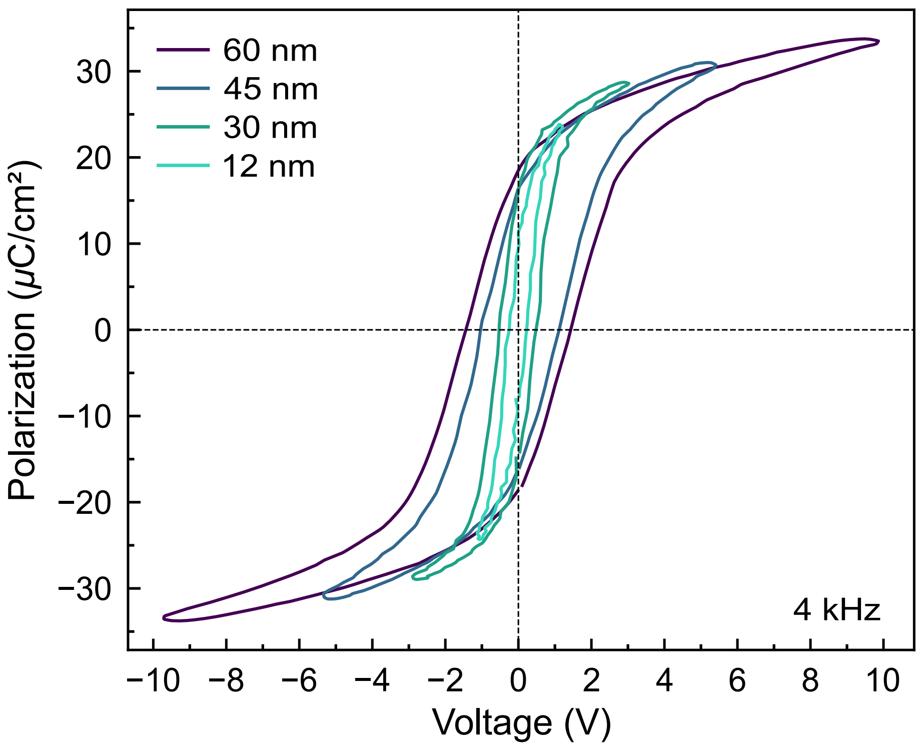


Figure S5. $P-V$ **profiles corresponding to the** $P-E$ **loops in Fig. 4c for BTO films of varying thickness.** All $I-E$ profiles are measured at 4 kHz on circular capacitors with an identical diameter of 30 µm. All films are free of imprint and leakage for applied voltages that significantly exceed the coercive field.

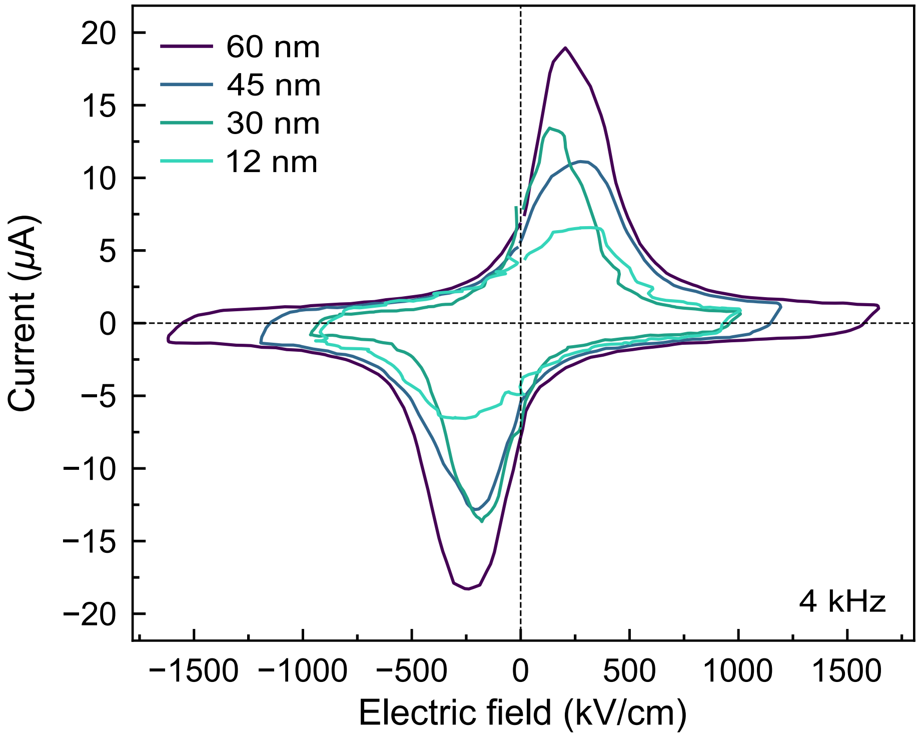


Figure S6. $I-E$ **profiles corresponding to the** $P-E$ **loops in Fig. 4c for BTO films of varying thickness.** All $I-E$ profiles are measured at 4 kHz on circular capacitors with an identical diameter of 30 μm. All films are free of imprint and leakage for applied voltages that significantly exceed the coercive field.

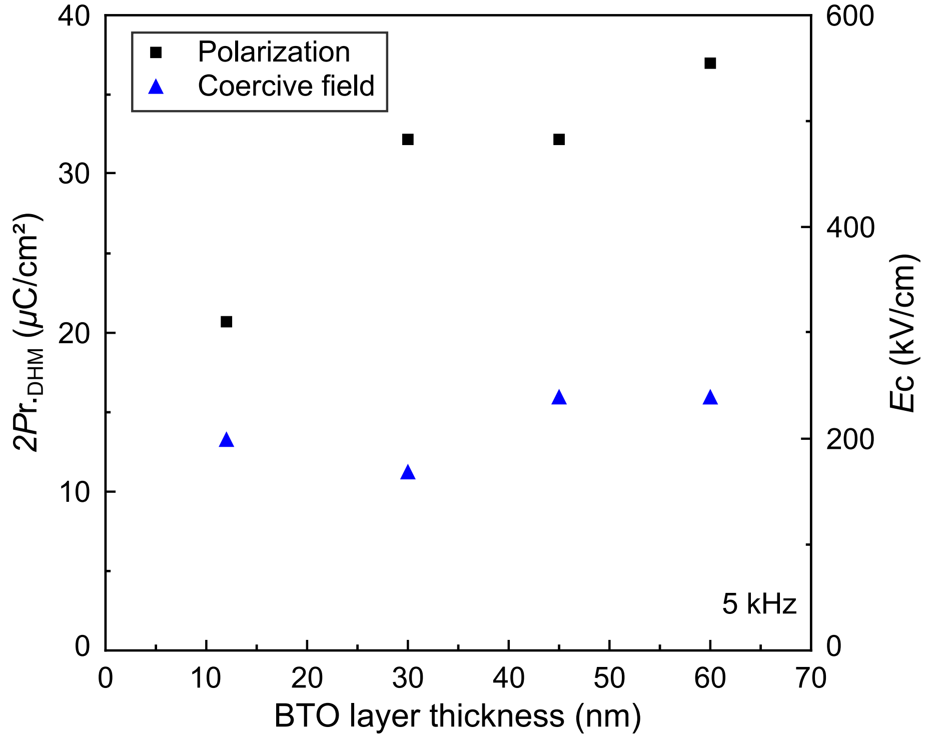


Figure S7. **Thickness dependence of remanent polarization ($2P_r$) and coercive field ($E_c$) of BTO films on Si.** With reducing film thickness, we observe a clear reduction of the remanent polarization and an increased depolarization effect. The coercive field, however, remains largely independent of film thickness, implying a reduction of the coercive voltage to continues down to a BTO film thickness of 12 nm.

Table S1. Literature overview of relevant ferroelectric metrics for BTO films grown on Si substrates.

| No. | Paper Title | Film Orientation | Thickness (nm) | $2P_r$ (μC cm$^{-2}$) | $E_c$ (kV cm$^{-1}$) | $V_c$ (V) | $V_{imprint}$ (V) | Measurement frequency | Authors |
|---|---|---|---|---|---|---|---|---|---|
| 1 | Nanoferroelectric domains in ultrathin $BaTiO_3$ films | Polycrystalline | 4 | 0.01 | 700 | 0.31 | 0.05 | 1 kHz | Drezner *et al.*[1] |
| 2 | Origin of compressive strain and phase-transition characteristics of thin $BaTiO_3$ films grown on $LaNiO_3$/Si substrates | Polycrystalline | 100 | 20.40 | 75.40 | 0.75 | 0.22 | 100 Hz–120 MHz | Qiao *et al.*[2] |
| 3 | Ultra-flat $BaTiO_3$ epitaxial films on Si(001) with large out-of-plane polarization | Epitaxial | 400 | 19.13 | 250.63 | 1.38 | 0.22 | 1−15 kHz | Scigaj *et al.*[3] |
| 4 | Coherent epitaxy of a ferroelectric heterostructure on a tri-layered buffer for integration into silicon | Epitaxial | 40 | 34.60 | 1097 | 4.39 | 0.14 | 1 kHz | Yamada *et al.*[4] |
| 5 | Fabrication and ferroelectric properties of $BaTiO_3$ thin films deposited on silicon substrate using PLD | Polycrystalline | 200 | 0.01 | 157.81 | 3.16 | 1.03 | 10 kHz | Dwivedi *et al.*[5] |
| 6 | Control of polar orientation and lattice strain in epitaxial $BaTiO_3$ films on silicon | Epitaxial | $103 \pm 9$ | 14.96 | $404 \pm 35$ | 4.16 | 0.21 | 150 Hz | Lyu *et al.*[6] |
| 7 | Enabling ultra-low-voltage switching in $BaTiO_3$ | Epitaxial | 100 | 31.05 | 40.01 | 0.16 | 0.18 | 1 kHz | Jiang *et al.*[7] |
| 8 | Achieving high ferroelectric polarization in ultrathin $BaTiO_3$ films on silicon | Polycrystalline | 35 | 31.22 | 1525.66 | 8.39 | 10 | 5 kHz | Bagul *et al.*[8] |
| 9 | This work | Epitaxial | 30 | 25.2 | 98.59 | 0.3 | $0.01 \pm 0.03$ | 1 kHz | Zhao *et al.* |

[1] Y. Drezner and S. Berger, J. Appl. Phys. **94**, 6774 (2003).

[2] L. Qiao and X. Bi, Phys. Status Solidi A **207**, 2511 (2010).

[3] M. Scigaj, N. Dix, I. Fina, R. Bachelet, B. Warot-Fonrose, J. Fontcuberta, and F. Sánchez, Appl. Phys. Lett. **102**, 112905 (2013).

[4] H. Yamada, Y. Toyosaki, and A. Sawa, Adv. Electron. Mater. **2**, 1500334 (2016).

[5] V. K. Dwivedi, Mater. Today Proc. **5**, 9132 (2018).

[6] J. Lyu, S. Estandía, J. Gazquez, M. F. Chisholm, I. Fina, N. Dix, J. Fontcuberta, and F. Sánchez, ACS Appl. Mater. Interfaces **10**, 25529 (2018).

[7] Y. Jiang, E. Parsonnet, A. Qualls, W. Zhao, S. Susarla, D. Pesquera, A. Dasgupta, M. Acharya, H. Zhang, T. Gosavi, C.-C. Lin, D. E. Nikonov, H. Li, I. A. Young, R. Ramesh, and L. W. Martin, Nat. Mater. **21**, 779-785 (2022).

[8] P. Bagul, H. Han, P. Lagrain, S. Sergeant, I. Hoflijk, J. Serron, O. Richard, T. Conard, J. Van Houdt, I. De Wolf, and S. R. C. McMitchell, Adv. Electron. Mater. **11**, 2400440 (2025).
